# Supplementary material for: Beyond Pass or Fail: Multi-Dimensional Benchmarking of Foundation Models for Goal-based Mobile UI Navigation
Source: arXiv:2501.02863 source file (2025-02-11)
Supplement: Supplementary file 1 [file appendix.tex]

\appendix
\section{Appendix}
